# Supplementary material for: The Responsible Foundation Model Development Cheatsheet: A Review of Tools & Resources
Source: arXiv:2406.16746 source file (2025-02-17)
Supplement: Supplementary file 1 [file 9a_appendix_sans_contributions.tex]

\section{Cheatsheet Samples}

In this portion of the appendix we have placed \textbf{samples} of the online cheatsheet, as examples of some of the content in each section.

% \vspace{-2mm}
\paragraph{Notations and Symbols}
The cheatsheet tables denote modalities and links with symbols, for brevity.
Modalities are indicated for text ~\TextCircle[0.75]{}, vision~\VisionCircle[0.75]{}, and speech ~\SpeechCircle[0.75].
We also provide hyperlinks for ArXiv \earxiv[1.2em][-0.4ex]\hspace{0.25em}, for Hugging Face objects \ehf[1.2em][-0.4ex]\hspace{0.25em}, for GitHub \egithub[1.2em][-0.4ex]\hspace{0.25em}, and for webpages \eweb[1.2em][-0.4ex]\hspace{0.25em}.

\tocless\subsection{Data Sourcing}

\begin{table}[H]
% % [inline block 0: 27 envs, 84042 chars -> data_tex | \begin{tabular}{@{}lllll@{}} \begin{tabular}{@{}p{\colOneSize}p{\colTwoSize}p{\colThreeSize}p{\colFourSize}@{}}...]

\end{table}
